# Supplementary material for: Opportunistic View Materialization with Deep Reinforcement Learning
Source: arXiv:1903.01363 source file (2019-03-04)
Supplement: Supplementary file 1 [file appendix.tex]

\section{Other Components}

\subsection{Candidate View Mining}
Naively, query level materialization with conventional cache policy might be enough for static query workloads. But in many situation it is not sufficient because queries might be generated from the same query template with different parameters. 
On the other hand, view candidates that are shared among different queries are often hand crafted by DBAs. Even with the help of design assisting tools, at the end of the day, it is the DBA who make the final decision. We believe a human-central process like this is usually expensive, largely depends on DBA's experience and does not scale. Most importantly, such an effort might only explore a small subset of the action space thus might fail to explore and exploit better views.

\begin{figure*}[!htbp]
    \centering
    \includegraphics[scale=0.55]{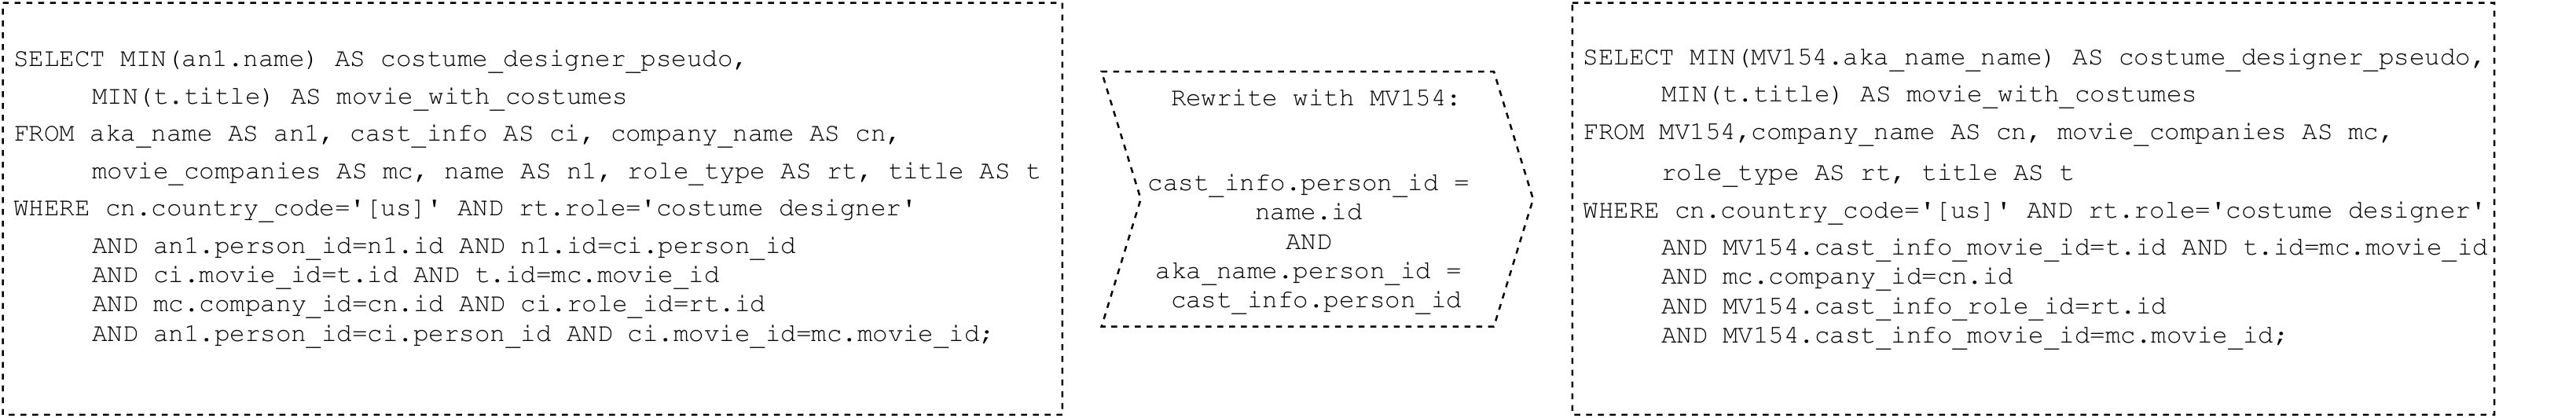}
    \caption{Rewrite JOB-8d}
    \label{8d}
\end{figure*}

We argue that an automated candidate view generation process combined with an intelligent view selection policy could be more scalable and could yield better result because: (1) such an automated process can explore larger action space to find better views candidates that were previously unexplored, (2) by offloading the view selection to another dedicating process we can maximize the benefit of good views and minimize the cost of bad views, (3) an intelligent view selection process like a RL algorithm does not rely on heuristics or experience therefore we could potentially benefit from views that were previously ignored.

% transitivity narrows down the action space, but still large enough for us to explore in our experiments.
In our system we implemented a view candidate miner based on join conditions (inner join). The idea is to mine the logical plans of previous queries to find the join conditions being used. Then given the two-table join conditions, we leverage the transitivity of joins and derive more complicated join conditions of n tables ($n > 2$). Each join condition represents a view candidate and the whole set of join conditions became our action space. An example of the mining process is given in Figure \ref{mining}.

In the experiments section, we demonstrate that the performance of our system boosted significantly by using the view candidates generated by our join-based miner.

\subsection{Join-Based Query Rewriter}

Given the join-based view candidates, our query rewriter implementation is straight forward. To determine whether a view can be used to rewrite a query, we simply go through the conditions in the where clause of the query to see if all the join conditions in the view has been covered by the query. If all the conditions in the view are covered, we first rename the relevant tables references in the query by the view name, then we get rid of the where conditions that are covered by the view. An example of rewriting query 8d from JOB is shown in Figure \ref{8d}.

We should note that in modern DBMS like Oracle, SQL Server, we take query rewriting as granted. I.e. we assume that once we have materialized a set of views, the DBMS or the query optimizer can decide which view to rewrite the query with then perform the rewriting. However, implementing a query rewriter is not a trivial task. Usually, in order to leverage sophisticated view candidates a lot of engineering efforts will be required to implement a query rewriter. This is also the case when we port our job-based rewriter to work with TPC-DS, due to the complexity of the TPC-DS queries and time constraint, we only used part of the TPC-DS queries in our experiments. 

\subsection{View Creation Policy}
Given several view candidates that can be applied to rewrite a query, we need to decide which view(s) to create. This is a challenging problem because (1) different views produce different benefit on different query/workload (2) maintenance cost of views vary, the benefit produced by a view might hardly exceeds its cost (3) the optimal view selection strategy might change given different constrains.

All factors mentioned above make this problem hard to trace and manage manually. But this is also an opportunity for RL techniques to make a difference. Given a RL agent that is trained with a cost aware reward function. We can simplify the complicated decision making process to be taking the action that is predicted by the agent to have the highest long term value. I.e. 

\[
a^* = \arg \max_{a \in A} Q(s,a) 
\]

Where $A$ is our action space, $s$ is current state, Q is the Q-function estimated by our RL algorithm.

In our implementation, our neural network take the features (state-action encoding) as input and output a number representing the value of taking action at current state. Every time we processed a query, we construct a matrix with relevant views (actions) and current state and ask the RL agent to batch process the whole matrix which give us the value of each pair. And the pair of highest value represent the view we should create (if the view does not already exist).
